# Supplementary material for: ContraGAN: Contrastive Learning for Conditional Image Generation
Source: arXiv:2006.12681 source file (2021-02-03)
Supplement: Supplementary file 1 [file FIgureA3.tex]

\begin{figure}[h!]
    
    \centering
    \includegraphics[scale=.45]{Supplement/Figures/pdf/FigureA3_num_classes.pdf}
    \caption{Change of \text{log}(FID) values as the number of classes increases. The proposed ContraGAN benefits from larger number of classes. Experiments are performed using Tiny ImageNet dataset.} 
    \label{FigureA3}
\end{figure}
