# Supplementary material for: ContraGAN: Contrastive Learning for Conditional Image Generation
Source: arXiv:2006.12681 source file (2021-02-03)
Supplement: Supplementary file 2 [file FigureA3_temp.tex]

\begin{figure}[h]
     \renewcommand\thefigure{A\arabic{figure}}
     \centering
     \begin{subfigure}[b]{0.48\textwidth}
         \centering
\includegraphics[width=\textwidth]{Supplement/Figures/pdf/FigureA3_num_classes.pdf}
         \caption{}
         \label{FigureA3}
     \end{subfigure}
     \hfill
     \begin{subfigure}[b]{0.48\textwidth}
         \centering
         \includegraphics[width=\textwidth]{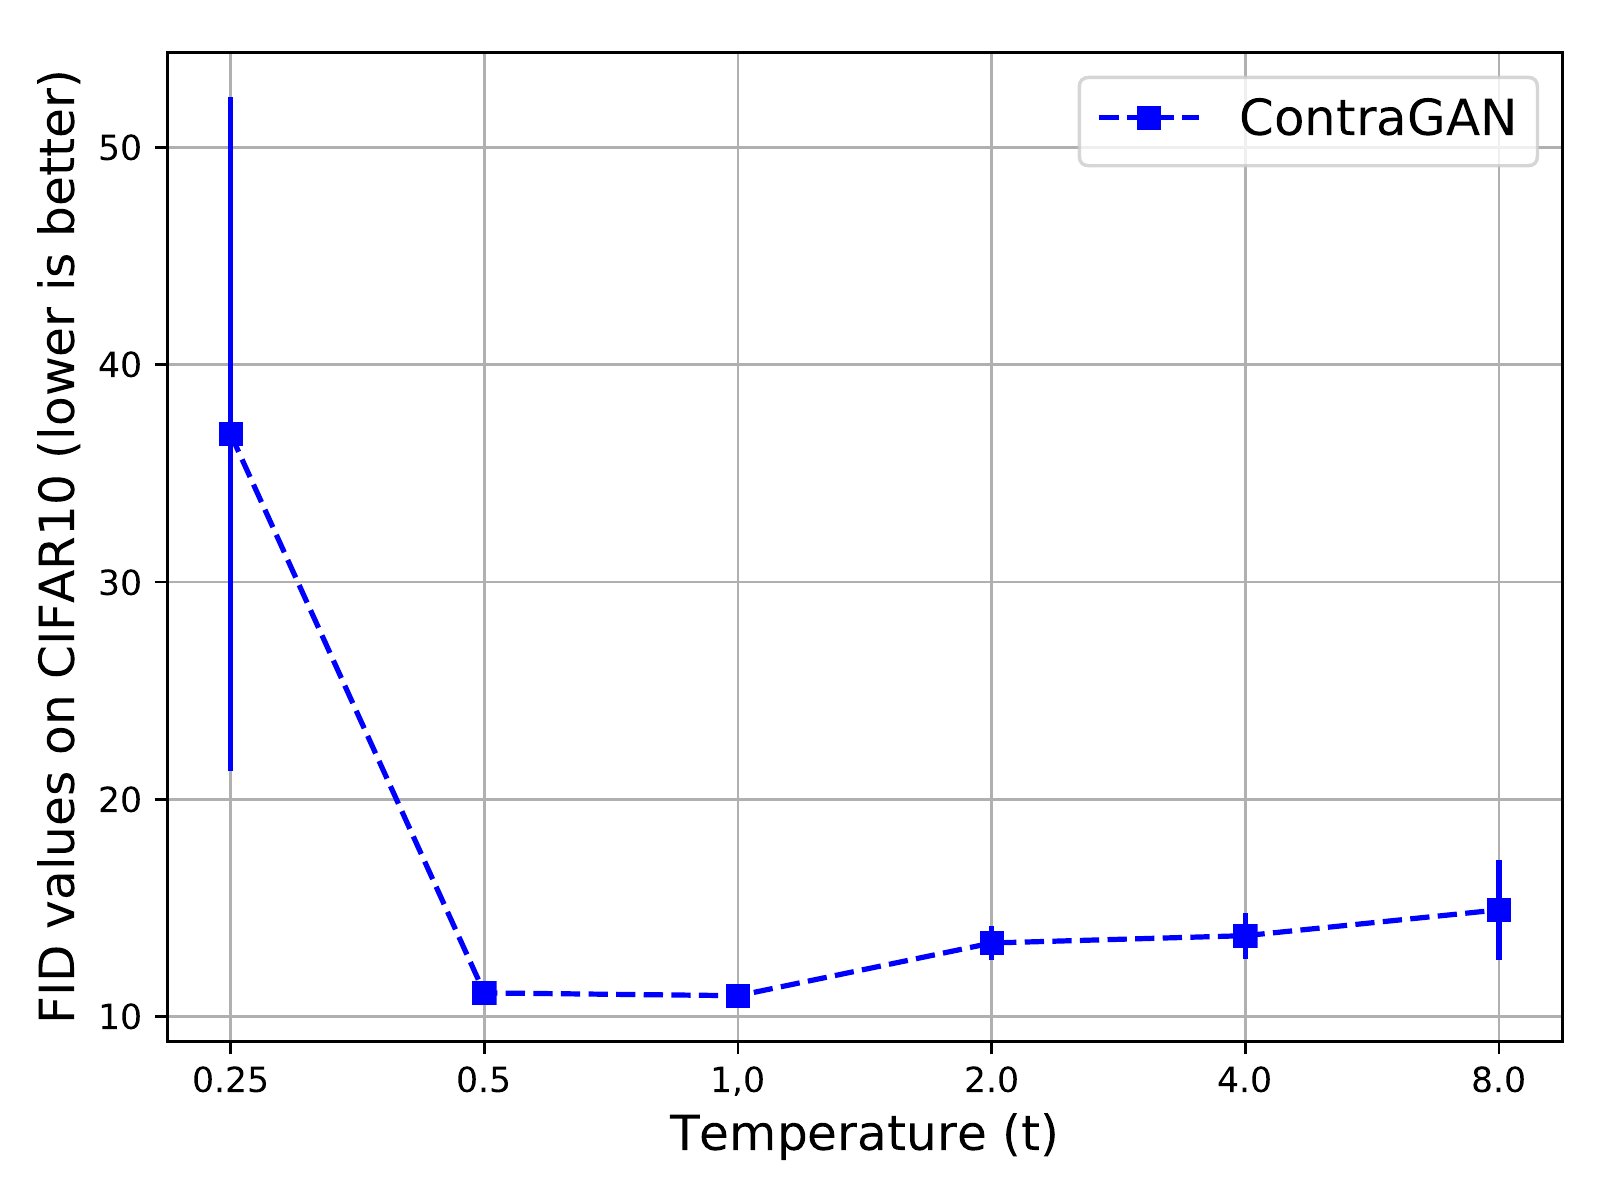}
         \caption{}
         \label{fig}
     \end{subfigure}
    \caption{(a) FID values of the ContraGAN with different projection layers and embedding dimensionalities. (b) the change in FID value when the experiments are conducted on the CIFAR10 and Tiny ImageNet dataset.
    The experiments (a) and (b) are conducted using the setting (D) described above. \jaesik{How about adding colors on the left vetical ticks and right vertical ticks?}}
    \label{figure3}
\end{figure}
